# Supplementary material for: Optimal Trade Execution with Uncertain Volume Target
Source: arXiv:1810.11454 source file (2021-09-14)
Supplement: Supplementary file 1 [file A-appendix.tex]

\section{Technical proofs}%
\label{sec:proofs}

\begin{proofalone}[\Cref{lemma:mean_variance_strategy_independent_of_volume}]
  Based on \eqref{eq:mean_variance_trading_cost} we have
  \begin{align*}
    \expe{ \Cost \pa{ \rquantb } }
    & =  
    \sum_{i=1}^{m} \gamma_{i} \rquant_{i} \pa{ \ftarget_{T} - \sum^{i}_{k=1} \rquant_{k} } 
    + \sum_{i=1}^{m} \pa{ \epsilon \abs{\rquant_{i}} + \frac{\eta_{i} \rquant_{i}^{2}}{\tau} }\\
    & =
    \sum_{i=1}^{m} \gamma_{i} \ystrat_{i} \pa{ 1 - \sum^{i}_{k=1} \ystrat_{k} } \ftarget_{T}^{2} 
    +  \sum_{i=1}^{m} \pa{ \epsilon \abs{y_{i} \ftarget_{T} }
    + \frac{\eta_{i} }{\tau_{i}} \pa{ \ystrat_{i} \ftarget_{T} }^2 }, \\
    \vari{\Cost(\rquantb)} & =
    \sum_{i=1}^{m} \tau_{i} \sigma_{i}^{2} \pa{ \ftarget_{T}
    - \sum^{i}_{k=1} \rquant_{k} }^2
    =
    \sum_{i=1}^{m} \tau_{i} \sigma_{i}^{2} \pa{ 1 - \sum^{i}_{k=1} \ystrat_k }^2\ftarget_{T}^2.
  \end{align*}
  Moreover,
  the optimal volumes $\rquantb^\star$ of Optimisation Problem~\eqref{eq:mean_variance_optimisation_problem} are positive if $\ftarget_{T} > 0$, which is assumed here \citep{Almgren2001}.
  Therefore,
  adding the non-negativeness constraint of the decision variables $\rquantb$ to Optimisation Problem~\eqref{eq:mean_variance_optimisation_problem} does not alter the optimal solution.
  Hence,
  one can replace $\sum_{i=1}^{m} \epsilon \abs{\rquant_{i}} $ by $ \sum_{i=1}^{m} \epsilon \rquant_{i} = \epsilon \ftarget_{T}$.
  As a consequence,
  all the terms in the objective function of Optimisation Problem~\eqref{eq:mean_variance_optimisation_problem} that depend on the decision variables $\ystratb$ are multiplied by $\ftarget_{T}^{2}$, 
  which means that $\ftarget_{T}$ has no impact on the optimal solution $\ystratb^{\star}$.
\end{proofalone}

\begin{proofalone}[\Cref{lemma:mean_CVaR_reproducibility_mean_variance_with_recourse}]%
  Let define $\bar{\ystratb}$ as $ \ystratb^{\star,t_0} > 0 $,
  the optimal solution of Optimisation Problem~\eqref{eq:mean_variance_optimisation_problem} at time~$t_0$,
  and
  $\bar{\betab} = \pa{ \bar{\beta}_{k,i} } \in \R^{m-1 \times m} $ 
  as the redistribution matrix parameter induced by this strategy $\ystratb^{\star,t_0}$,
  \ie the matrix defined as follows:
  \begin{equation}
    \bar{\beta}_{k,i} \pa{ \ystratb^{\star,t_0} } =
    \begin{cases}
      0 & \text{ if } i \leq k, \\
      \frac{\ystrat^{\star,t_0}_{i}}{\sum_{r=k+1}^{m}{\ystrat^{\star,t_0}_{r}}} ,
	& \text{ otherwise. }
    \end{cases}
  \end{equation}
  Indeed,
  using the fact that $\sum_{i=1}^{m} \ystrat^{\star,t_{0}}_{i} = 1$,
  one has that the volumes $\rquantb^{rec}$ are given by
  \begin{align}
    \rquant_{1}^{rec} & = \ystrat^{\star,t_{0}}_{1} \rtarget_{0}, \\
    \rquant_{2}^{rec} &
    =
    \frac{\ystrat^{\star,t_{0}}_{2}}{\sum_{r=2}^{m} \ystrat^{\star,t_{0}}_{r}} \pa{\rtarget_{0} + \rupdate_{1} - \ystrat^{\star,t_{0}}_{1} \rtarget_{0}}
    =
    \frac{\ystrat^{\star,t_{0}}_{2}}{1 - \ystrat^{\star,t_{0}}_{1}} \pa{ \pa{ 1 - \ystrat^{\star,t_{0}}_{1} } \rtarget_{0} + \rupdate_{1} } \\
  &
    =
    \ystrat^{\star,t_{0}}_{2} \rtarget_{0} + 
    \frac{\ystrat^{\star,t_{0}}_{2}}{1 - \ystrat^{\star,t_{0}}_{1}} \rupdate_{1} \\
    \rquant_{3}^{rec} &
    =
    \frac{\ystrat^{\star,t_{0}}_{3}}{\sum_{r=3}^{m} \ystrat^{\star,t_{0}}_{r}} \pa{
  \rtarget_{0} + \rupdate_{1} + \rupdate_{2}
  - \ystrat^{\star,t_{0}}_{1} \rtarget_{0}
  - \ystrat^{\star,t_{0}}_{2} \rtarget_{0}
  - \frac{\ystrat^{\star,t_{0}}_{2}}{1 - \ystrat^{\star,t_{0}}_{1}} \rupdate_{1}
    } \\
  &
    = 
    \ystrat^{\star,t_{0}}_{3} \rtarget_{0}
    + \frac{\ystrat^{\star,t_{0}}_{3}}{1 - \ystrat^{\star,t_{0}}_{1}} \rupdate_{1}
    + \frac{\ystrat^{\star,t_{0}}_{3}}{1 - \ystrat^{\star,t_{0}}_{1} - \ystrat^{\star,t_{0}}_{2}} \rupdate_{2} \\
  & \vdots \nonumber \\
    \rquant_{i}^{rec} &
    = 
    \ystrat^{\star,t_{0}}_{i} \rtarget_{0}
    + \sum_{k=1}^{i-1} 
    \pa{
  \frac{\ystrat^{\star,t_{0}}_{i}}{ 1 - \sum_{r=1}^{k} \ystrat^{\star,t_{0}}_{r}}
    } \rupdate_{k}. \label{eq:rec_volume_i}
  \end{align}
  Then, 
  if one uses the notations $\bar{\ystratb}$ and $\bar{\betab}$,
  one obtains
  \begin{equation}
    \rquant_{i}^{rec}
    =
    \bar{\ystrat}_{i} \rtarget_{0}
    + \sum_{k=1}^{i-1} 
    \pa{
      \frac{ \pa{1 - \sum_{r=1}^{k} \bar{\ystrat}_{r} } \bar{\ystrat}_{i} + \bar{\ystrat}_{i} \pa{\sum_{r=1}^{k} \bar{\ystrat}_{r} } }{ 1 - \sum_{r=1}^{k} \bar{\ystrat}_{r}}
    } \rupdate_{k}
    = 
    \bar{\ystrat}_{i} \rtarget_{0}
    + \sum_{k=1}^{i-1} 
    \pa{
      \bar{\ystrat}_{i}
      +
    \bar{\beta}_{r} \sum_{r=1}^{k} \bar{\ystrat}_{r} } \rupdate_{k},
  \end{equation}
  which is the expression of trading volumes given by \Cref{eq:relation_volume_proportion}.
\end{proofalone}
